# Supplementary material for: Grain Boundary Structures and Collective Dynamics of Inversion Domains in Binary Two-Dimensional Materials
Source: arXiv:1705.07822 source file (2017-05-22)
Supplement: Supplementary file 1 [file hBN_GBs_arXiv_supp.pdf]

# Supplemental Material
# Grain Boundary Structures and Collective Dynamics of Inversion Domains in Binary Two-Dimensional Materials

Doaa Taha,[1] S. K. Mkhonta,[1,2] K. R. Elder,[3] and Zhi-Feng Huang[1]

[1] *Department of Physics and Astronomy, Wayne State University, Detroit, Michigan 48201, USA*
[2] *Department of Physics, University of Swaziland, Private Bag 4, Kwaluseni M201, Swaziland*
[3] *Department of Physics, Oakland University, Rochester, Michigan 48309, USA*

## I. BINARY PFC MODEL AND PHASE DIAGRAM

The binary phase field crystal (PFC) model introduced in this work can be connected to classical density functional theory (DFT). Following the derivation procedure of Ref. [1] based on classical dynamic DFT, we expand two- and three-point direct correlation functions $C_{ij}^{(2)}$ and $C_{ijk}^{(3)}$ $(i,j,k = A, B)$ in Fourier space, i.e., $\hat{C}_{ij}^{(2)}(q) = -\hat{C}_0^{ij} + \hat{C}_2^{ij} q^2 - \hat{C}_4^{ij} q^4 + \cdots$ and $\hat{C}_{ijk}^{(3)}(\boldsymbol{q},\boldsymbol{q}') \simeq \hat{C}_{ijk}^{(3)}(\boldsymbol{q}=\boldsymbol{q}'=0) = -\hat{C}_0^{ijk}$, and obtain the resulting free energy functional. Rescaling spatial and temporal scales leads to the dimensionless free energy functional given in Eq. (2) of the main text, i.e.,

$$\mathcal{F} = \int d\boldsymbol{r} \left[ -\frac{1}{2}\epsilon_A n_A^2 + \frac{1}{2} n_A \left(\nabla^2 + q_A^2\right)^2 n_A - \frac{1}{3} g_A n_A^3 + \frac{1}{4} n_A^4 - \frac{1}{2}\epsilon_B n_B^2 + \frac{\beta_B}{2} n_B \left(\nabla^2 + q_B^2\right)^2 n_B - \frac{1}{3} g_B n_B^3 + \frac{1}{4} v n_B^4 \right.$$
$$\left. + \alpha_{AB} n_A n_B + \beta_{AB} n_A \left(\nabla^2 + q_{AB}^2\right)^2 n_B + \frac{1}{2} w n_A^2 n_B + \frac{1}{2} u n_A n_B^2 \right], \tag{1}$$

where the rescaled parameters are expressed in terms of Fourier expansion coefficients of two- and three-point correlation functions, that is,

$$\epsilon_{A(B)} = (B^x_{A(B)} - B^l_{A(B)})/B^x_A, \;\; B^x_A = \frac{\rho_l^A \, {\hat{C}_2^{AA}}^2}{4\hat{C}_4^{AA}}, \;\; B^l_A = 1 + \rho_l^A \hat{C}_0^{AA}, \;\; B^x_B = \frac{\rho_l^B \, {\hat{C}_2^{BB}}^2}{4\hat{C}_4^{BB}}, \;\; B^l_B = 1 + \rho_l^B \hat{C}_0^{BB},$$
$$q_A = 1, \;\; q_B = \sqrt{\frac{\hat{C}_4^{AA}\hat{C}_2^{BB}}{\hat{C}_4^{BB}\hat{C}_2^{AA}}}, \;\; q_{AB} = \sqrt{\frac{\hat{C}_4^{AA}\hat{C}_2^{AB}}{\hat{C}_4^{AB}\hat{C}_2^{AA}}}, \;\; \beta_B = \frac{\rho_l^B \hat{C}_4^{BB}}{\rho_l^A \hat{C}_4^{AA}}, \;\; \beta_{AB} = \frac{\hat{C}_4^{AB}}{\hat{C}_4^{AA}},$$
$$g_A = \frac{\sqrt{3}}{2}\left(\hat{C}_0^{AA} + \rho_l^A \hat{C}_0^{AAA}\right) \Big/ \sqrt{B^x_A \hat{C}_0^{AAA}}, \;\; g_B = \frac{\sqrt{3}}{2}\left(\hat{C}_0^{BB} + \rho_l^B \hat{C}_0^{BBB}\right) \Big/ \sqrt{B^x_A \hat{C}_0^{AAA}}, \;\; v = \frac{\hat{C}_0^{BBB}}{\hat{C}_0^{AAA}},$$
$$\alpha_{AB} = \frac{\hat{C}_4^{AA}}{{\hat{C}_2^{AA}}^2}\left(4\hat{C}_0^{AB} - {\hat{C}_2^{AB}}^2 / \hat{C}_4^{AB}\right), \;\; w = \frac{\sqrt{3}\rho_l^A \hat{C}_0^{AAB}}{\sqrt{B^x_A \hat{C}_0^{AAA}}}, \;\; u = \frac{\sqrt{3}\rho_l^A \hat{C}_0^{ABB}}{\sqrt{B^x_A \hat{C}_0^{AAA}}}, \tag{2}$$

with $\rho_l^{A(B)}$ the reference state density of A(B) component. In Eq. (1) of PFC free energy functional, the $\alpha_{AB}$ term would favor the occupation of A(B) minima by B(A) maxima and prevent the overlap of A and B atomic sites. The last two terms (i.e., $w$ and $u$ terms) would allow the overlap of A and B minima but not necessarily B(A) maxima on A(B) minima. These two terms are important for the stabilization of honeycomb structure, given the vacancy position (without either A or B site) in the center of a honeycomb ring. Without these 2 stabilizing terms some other phases such as the binary face-centered square could also form and coexist with the binary honeycomb phase [2].

From this binary PFC model we have identified 7 two-dimensional (2D) phases and the coexistence between them, as determined by the coupling between $n_A$ and $n_B$ fields. These include binary honeycomb (BH, with both A and B triangular sublattices), binary stripe (BS, with stripe phase of both A and B sublattices), elongated triangular A & stripe B (ETASB), elongated triangular B & stripe A (ETBSA), triangular A & inverse triangular B (TAHB), triangular B & inverse triangular A (TBHA), and binary homogeneous (BHom) phases. Some examples of defected states obtained from numerical simulations of the PFC model equations are shown in Fig. S1.

To calculate the phase diagram, we follow standard thermodynamics and determine the phase boundaries for the coexistence between any two phases via the conditions of equal chemical potentials and equal pressure. We also identify the stability diagram giving the phase of lowest free energy in each regime of the parameter space. An example of $n_{A0}$–$n_{B0}$ cross-section plane of stability and phase diagrams at $\epsilon_A = \epsilon_B = 0.3$ is shown in Fig. S2. The model parameters used are $q_A = q_B = q_{AB} = 1$, $\alpha_{AB} = 0.5$, $\beta_{AB} = 0.02$, $g_A = g_B = 0.5$, $w = u = 0.3$, and $\beta_B = v = 1$.

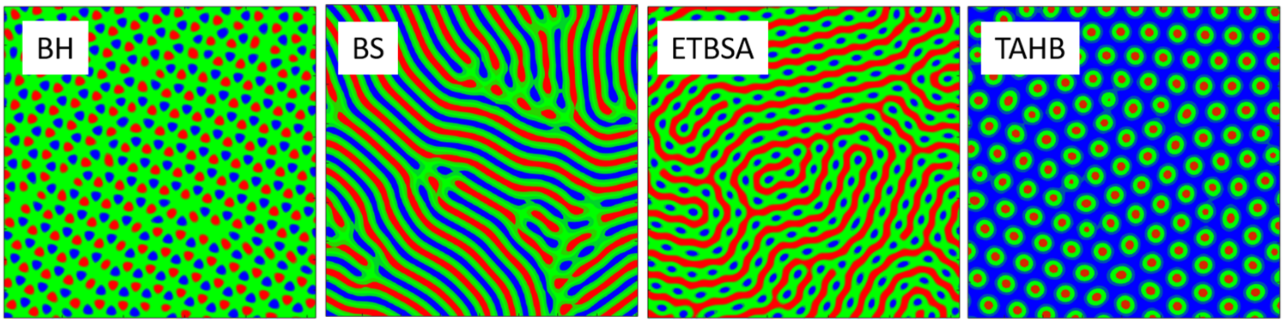


FIG. S1. Sample simulation results obtained from random initial condition, showing binary honeycomb (BH), binary stripe (BS), elongated triangular B & stripe A (ETBSA), and triangular A & inverse triangular B (TAHB) phases with defects, as taken from a portion of the simulation box.

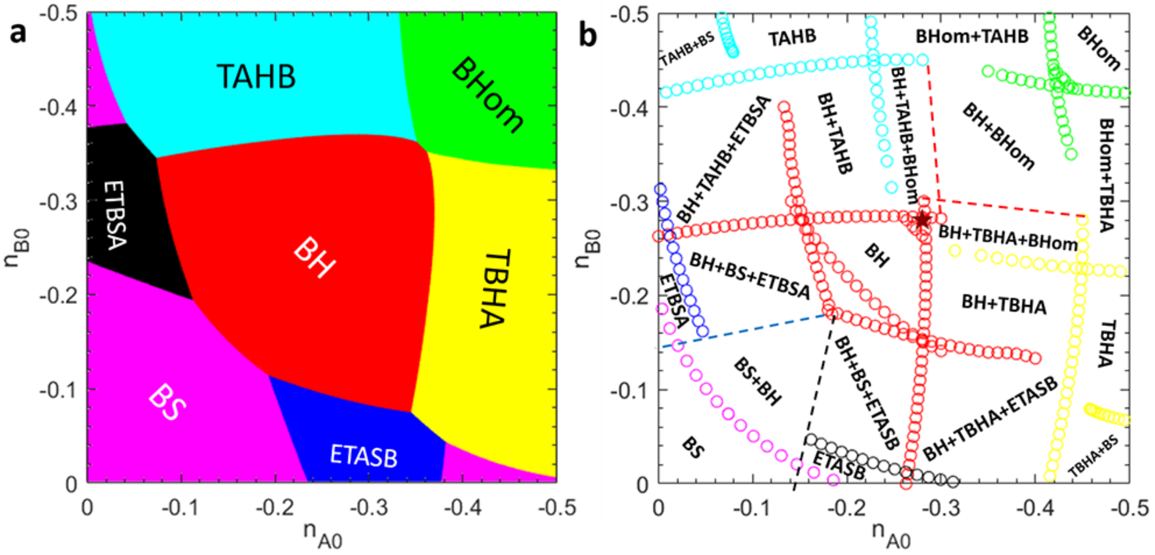


FIG. S2. (a) Stability diagram and (b) phase diagram of the binary PFC model in the cross-section plane of $n_{A0}$ vs $n_{B0}$ at $\epsilon_A = \epsilon_B = 0.3$, showing binary honeycomb (BH), binary homogeneous (BHom), binary stripe (BS), elongated triangular A & stripe B (ETASB), elongated triangular B & stripe A (ETBSA), triangular A & inverse triangular B (TAHB), and triangular B & inverse triangular A (TBHA) phases as well as their coexistent regimes. The star indicates the location of the parameter space ($n_{A0} = n_{B0} = -0.28$) used in the GBs study of the main text.

This setup of symmetric AB parameters (e.g., $\epsilon_A = \epsilon_B$, $g_A = g_B$, $w = u$, and $v = 1$) is used for the simulation of h-BN systems, given the similar roles of B and N components in the formation and dynamics of binary honeycomb phase. When modeling other materials usually with asymmetric roles of components, this assumption would no longer apply and different sets of model parameters should be chosen. This would in principal lead to different phase diagram and structural properties. Also as stated in the main text, in this binary PFC model there are two factors pivotal to the determination of model parameters and terms: The first one is crystalline symmetry (including lattice length scales), while the second one is specific for binary compounds of sublattice ordering, i.e., the heteroelemental A-B neighboring (bond) is favored energetically as compared to homoelemental A-A or B-B ones.

In addition, in this 2D study the out-of-plane deformations are not incorporated as they are assumed to be of secondary effect during epitaxial growth due to the substrate constraint of 2D material monolayers. To estimate the impact of out-of-plane deformations on our results, we note that even for free-standing monolayers, first-principles DFT calculations (e.g., Ref. [3] for h-BN and Ref. [4] for graphene) have shown that there is little buckling for large angle boundaries that contain a large concentration of dislocations. For the case of epitaxial overlayers, recent experiments showed that despite the weak film-substrate interaction, the substrate is able to effectively constrain the vertical corrugation of monolayer; for example, the flattening of out-of-plane warping was observed in defected h-BN sheets grown on metallic substrate [5]. Thus for small misorientation angles in epitaxial monolayers, grain boundary

energies are expected to slightly decrease due to the relaxation along the vertical direction, while our results for high-angle boundaries, particularly those of inversion domains, should remain unchanged due to their structure planarity.

## II. MODEL PARAMETERIZATION

All the parameters and variables given above for the PFC model are dimensionless. Thus the model needs to be parameterized and fitted for real 2D materials like h-BN, so that the calculated physical quantities can be compared to properties of real materials. As shown in Eq. (2), all the parameters in our PFC model can be connected to and expressed in terms of two- and three-point direct correlation functions of classical DFT, and thus can be connected to AB (or BN) atomic interactions. In principle we can then quantitatively determine the model parameters by fitting the direct correlation functions calculated from molecular dynamics (MD). This procedure has been applied to the single-component metallic system with well-studied MD data. The situation for 2D graphene-type materials is much more complicated, given that different versions of MD potentials often yield very different results. For example, a very recent study [6] attempted to quantitatively identify grain boundary energies and defect core structures of graphene using PFC models, MD, and first-principles DFT. The calculations involving 2 different MD potentials (AIREBO vs Tersoff) and a DFT package produced quite large quantitative deviations of grain boundary energies although showing similar defect core structures. The quantitative parameterization of PFC model for 2D materials is then hindered by this discrepancy between outcomes of atomistic calculations.

Given these constraints, in this study we focus on an alternative way of model parameterization for h-BN, i.e., through first constricting the parameters based on lattice symmetry and the relation between binary components as described in Sec. I, and then matching to length and energy scales of h-BN. The rationale of this approach can be partially justified by a recent work combining MD and first-principles DFT calculations and experiments [7], which showed similar detailed defect core structures and grain boundary behavior for graphene and hexagonal silica although they have very different bonding characteristics, demonstrating the pivotal role of lattice symmetry.

### Elastic properties

We first need to identify the elastic properties of the binary honeycomb phase, which will be used in parameterizing the PFC model. We follow the standard procedure by expanding the PFC free energy functional in terms of the linear strain tensor. In the limit of small deformation the PFC elastic constants of binary honeycomb phase are given by $C_{11} = C_{22}$ and $C_{12} = C_{44} = C_{11}/3$. This leads to a 2D bulk modulus $B = (C_{11} + C_{12})/2 \equiv \alpha/2$, shear modulus $\mu = C_{44} = \alpha/4$, and Young's modulus $Y_2 = 4B\mu/(B + \mu) = 2\alpha/3$. Values of these elastic constant can be calculated via determining $\alpha$ from direct numerical simulations of the full PFC equations. This is based on bulk deformation of a single crystal which gives the expansion of free energy density $f = \mathcal{F}/\mathcal{A}$ (with area $\mathcal{A}$) as [8]

$$f = f_0 + \alpha\zeta^2 + \cdots , \tag{3}$$

where $f_0$ is the equilibrium free energy density and the strain $\zeta = (a_x - a_0)/a_0$, with $a_x = 2\pi/q_x$ ($q_x = \sqrt{3}q/2$) and $a_0$ the equilibrium lattice constant. Numerically the bulk deformation is imposed by changing the numerical grid spacings $\Delta x$ and $\Delta y$, while keeping the constraint of periodic boundary conditions, i.e., the system size $l_x = L_x\Delta x = n_x a_x$ and $l_y = L_y\Delta y = n_y a_y$ where $n_x$, $n_y$ are integers and $a_y = 4\pi/q$ for the single crystal of honeycomb lattice. For the model parameters given in Sec. I and also $\epsilon_A = \epsilon_B = 0.3$, $n_{A0} = n_{B0} = -0.28$, our numerical calculations of free energy minimization and the fitting to Eq. (3) give $\alpha = 1.0755$, with the equilibrium parameters $q = 0.9875$, $q_x = 0.8552$, $\Delta x = 0.8035$, and $\Delta y = 0.8043$ for $L_x = 512$, $L_y = 886$, and $n_x = n_y = 56$.

### Parameterization for energy and length scales

In the following process of model parameterization we use the values of model parameters given above for equilibrium binary honeycomb phase, and label all the dimensional quantities in real units with superscript "$d$". Given the lattice constant $a_x = 2\pi/q_x$ in PFC and $a_0^d = 2.51$ Å for h-BN, a dimensionless length $l$ in 2D PFC is matched to a dimensional one $l^d$ of h-BN material via

$$l^d/l = a_0^d/a_x = a_0^d/(2\pi/q_x) = 0.342 \text{ Å}. \tag{4}$$

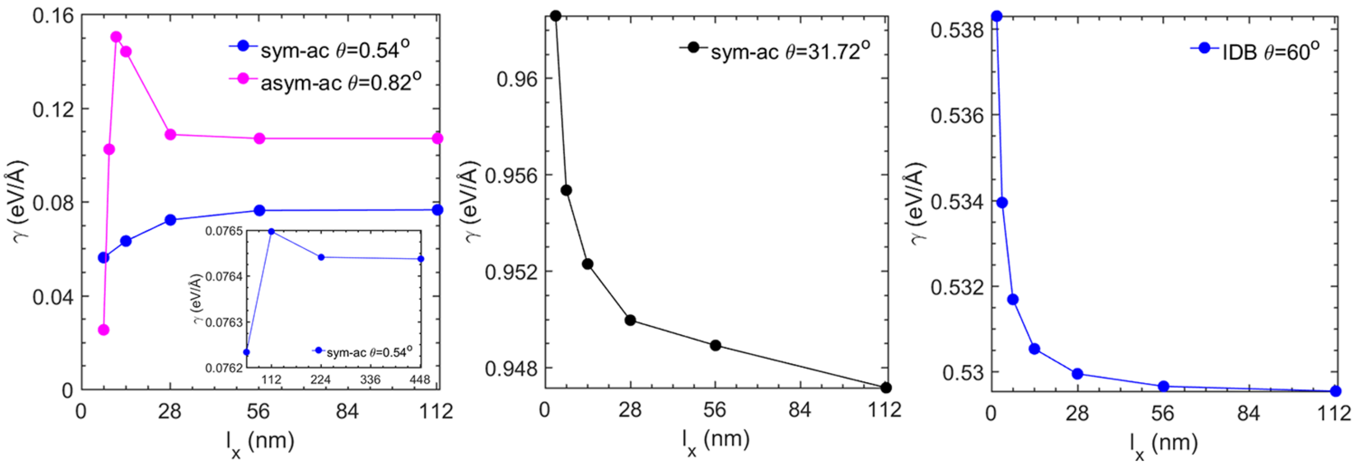


FIG. S3. Finite size effects in the GB energy calculation. Left: $\gamma$ vs $l_x$ for $\theta = 0.54^\circ$ (sym-ac, in both main panel and the inset, with $l_y = 53$ nm) and $\theta = 0.82^\circ$ (asym-ac, with $l_y = 70$ nm); Middle: $\theta = 31.72^\circ$ (sym-ac, with $l_y = 28.5$ nm); Right: $60^\circ$ inversion domain boundary (IDB, with 4|8 dislocation core structure and $l_y = 24.4$ nm).

Thus in this work the smallest simulation box of $L_x \times L_y = 512 \times 512$ corresponds to size $L_x\Delta x^d \times L_y \Delta y^d = 14.1$ nm $\times$ 14.1 nm, and the largest simulation size of $32768 \times 10010$ corresponds to 0.9 $\mu$m $\times$ 0.3 $\mu$m.

To identify the energy scale $c_0$ defined by $\mathcal{F}^d = c_0 \mathcal{F}$, we note from Eq. (3) that $f^d/f = Y_2^d/Y_2 = Y^d a_z^d/Y_2$, where $a_z^d = 3.33$ Å is the vertical layer spacing of h-BN. This yields $Y^d a_z^d / Y_2 = (\mathcal{F}^d/\mathcal{A}^d)/(\mathcal{F}/\mathcal{A}) = c_0 (a_x/a_0^d)^2$, and thus a PFC energy unit is determined by

$$c_0 = \frac{Y^d}{Y_2}\left(\frac{a_0^d}{a_x}\right)^2 a_z^d = \frac{3Y^d}{2\alpha}\left(\frac{a_0^d}{a_x}\right)^2 a_z^d = 2.74 \text{ eV}, \tag{5}$$

given the h-BN parameters of Young's modulus $Y^d = 810$ GPa, lattice constant $a_0^d$, and $a_z^d$.

In our grain boundary (GB) simulations, each initial configuration comprises two parallel interfaces (i.e., GBs) that are perpendicular to the $x$ direction, separating two misoriented single-crystalline regions. The GB energy $\gamma$ (per unit length) is then calculated via

$$\gamma = \frac{\mathcal{F} - \mathcal{F}_0}{2l_y} = \frac{l_x}{2}(f - f_0), \tag{6}$$

where $\mathcal{F}_0$ is the equilibrium free energy of the corresponding single-crystal system, $l_x = L_x \Delta x$, and $l_y = L_y \Delta y$. From Eqs. (4) and (5), the PFC GB energy unit is given by $c_0 a_x / a_0^d = 8.0$ eV/Å for h-BN.

## III. GRAIN BOUNDARY SIMULATIONS AND FINITE SIZE EFFECTS

Large enough system sizes are needed in the grain boundary computation due to artifacts of finite size effects. The two GBs in a simulation box need to be separated far enough from each other, to avoid any coupling between them as a result of long-range elastic interaction. Grain boundaries that are too close together tend to lead to an under- (over-) estimation of the GB energy for small (large) misorientations as shown in Fig. S3. For large-angle grain boundaries the elastic interaction of nearby boundaries tends to increase $\gamma$, while for small-angle boundaries the long-range elastic strains are not accounted for if the boundaries are too close to each other, given that the strain energy extends over a range increasing with the distance between dislocation cores along the boundary and GBs of smaller angle correspond to larger spacing between dislocation cores. There are rather limited finite size effects along the GB direction (i.e., for $l_y$), provided that large enough $l_y$ is used to avoid any cutoff of dislocation core structures particularly for the sinuous, irregularly-spaced defect arrays in asym-ac GBs.

More sample GB configurations obtained from our PFC simulations are presented in Fig. S4, including some examples of symmetrically tilted GBs (from both sym-ac and sym-zz setups) and asymmetrically tilted armchair GBs (asym-ac) that are of sinuous feature.

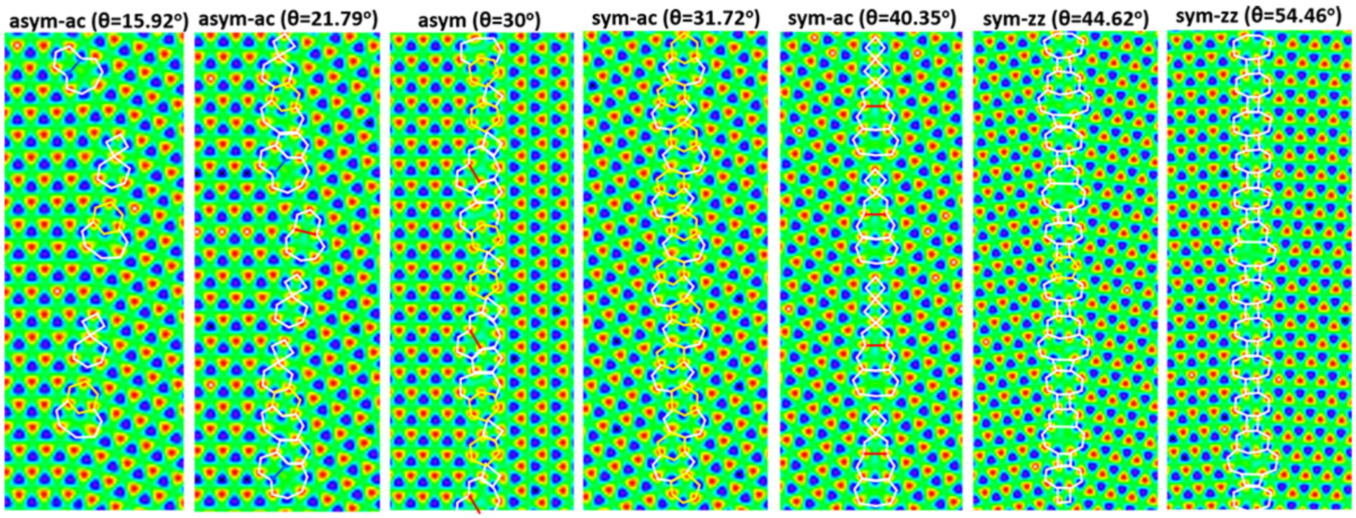


FIG. S4. Sample structures for symmetrically or asymmetrically tilted GBs at various misorientation angles $\theta$, starting from either armchair (ac) or zigzag (zz) direction.

## IV. PARAMETER DEPENDENCE OF RESULTS

To further address the reliability of our approach and the degree of parameter independence of our results, we have conducted a large number of additional simulations with varying model parameters, particularly for high angle boundaries. All show similar results.

(i) To systematically investigate the structure and energy of 60° inversion domain boundaries (IDBs) which are of current interest, we consider the cases of a) varying values of $\epsilon_A = \epsilon_B$ (e.g., $= 0.1, 0.3, 0.5$, similar to temperature effect), b) varying $g_A = g_B$ values (e.g., $= 0, 0.5, 1$), c) changing values of $\alpha_{AB}$ and $w = u$, and d) also varying $n_{A0} = n_{B0}$ values. All these gave similar results for the defect core structures and grain boundary energy sequence; i.e., 4|8 structure is always the lowest energy state of 60° boundary, while for other higher-energy metastable IDB structures, the $\gamma$ values for 8|8 and 4|4 structures are usually quite close to each other. Also at lower (higher) atomic densities $n_{A0}$, $n_{B0}$ while keeping the other parameters the same, which corresponds to being closer to (further away from) the coexistence between solid and homogeneous states, the defect structures that are vacancy-rich (e.g., 8|8, Z6-I, AT12) are more (less) easily stabilized as compared to compacted structures (e.g., 4|4, AT8, Z6-II).

(ii) We have examined the dynamics of grain growth for 60° inversion domains for different sets of model parameters (e.g., varying $\epsilon_A = \epsilon_B$, varying $g_A = g_B$, or varying $w = u$), with some results given in Fig. S5. The domain evolution and shrinking processes are very similar to that in Fig. 4 of the main text, all showing the mechanisms of collective atomic dynamics at the boundaries and junctions and also linear regimes of grain area shrinkage for 4|8 boundaries as in Fig. 4c.

In addition, all the GB energies ($\gamma$ values in Fig. 2 of the main text) calculated from our PFC model are within the range of first-principles DFT results [3]. Specifically, for 4|8 60° IDB the DFT calculation yielded $\gamma \sim 0.43$ eV/Å for h-BN [3], while our PFC result (in Fig. 3 of the main text) gives $\gamma = 0.53$ eV/Å. This $\sim 20\%$ difference could be viewed as being in reasonably good agreement, given that DFT is for zero-temperature calculations and in the case of graphene the difference between MD and DFT results of $\gamma$ would be much larger (MD values are mostly larger than those of DFT [6]).

## V. GRAIN GROWTH DYNAMICS

Three supplemental movies are provided to show the dynamic process of grain coalescence and inversion domain evolution, including one corresponding to Fig. 4 of the main text and additional two with different types of inversion domain boundaries. For the 2nd movie where one of the polygon inversion domains shows slower shrinkage rate and growth stagnation, we have also tracked the atomic site number $N$ inside the domain as a function of time $t$, with result presented in Fig. S6.

In our study of inversion domain dynamics, although there is no lattice plane misorientation across the inversion

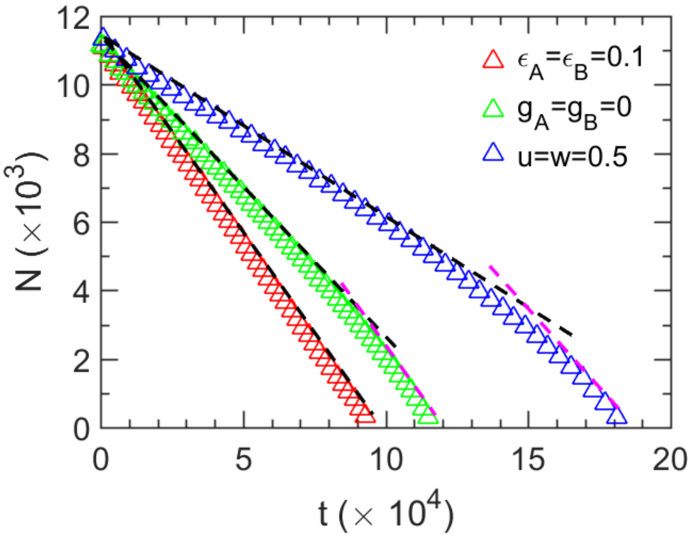


FIG. S5. Additional results of inversion domain shrinking, for atomic site number $N$ of a triangle inversion domain vs time $t$. Three sets of parameters different from those of the main text are used: (1) $\epsilon_A = \epsilon_B = 0.1$, $g_A = g_B = 0.5$, $\alpha_{AB} = 0.5$, $w = u = 0.3$, (2) $g_A = g_B = 0$, $\epsilon_A = \epsilon_B = 0.3$, $\alpha_{AB} = 0.5$, $w = u = 0.3$, and (3) $w = u = 0.5$, $\epsilon_A = \epsilon_B = 0.3$, $g_A = g_B = 0.5$, $\alpha_{AB} = 0.5$.

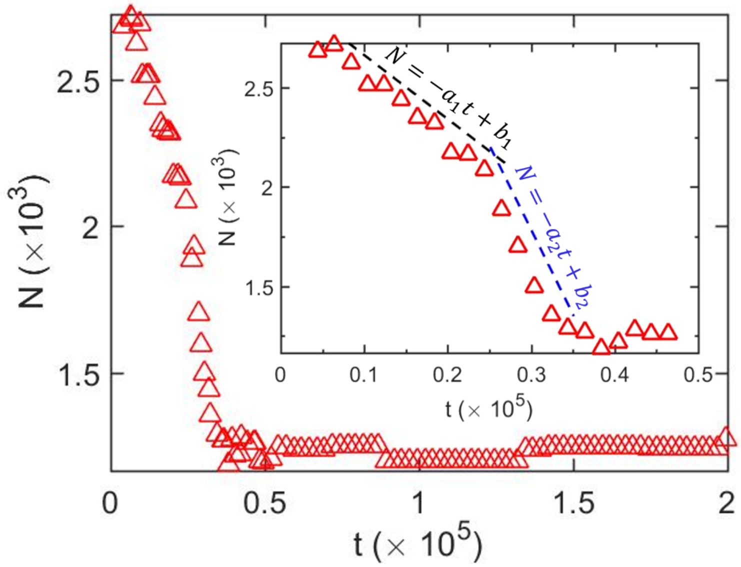


FIG. S6. Atomic site number $N$ as a function of time $t$, for time evolution of the lower-left polygon inversion domain in supplemental movie 2 which becomes stagnant at late time. The result of early-time domain shrinking is enlarged and presented in the inset, which can be fitted into two linear regimes $N = -0.032t + 2.88 \times 10^3$ and $N = -0.085t + 4.13 \times 10^3$.

domain boundaries, if using the notation in Ref. [9] the Burgers vector for 4|8 dislocation pairs is always perpendicular to the boundary line during the domain shrinking process of Fig. 4. Since the domain boundary motion is collective and rigidly inward, through the simultaneous evolution and transformation of the boundary defect rings mediated via the corner defects, it involves the process of dislocation glide but not climb. This dynamic process predicted here should then be readily reproduced in MD simulations with similar system setup.

Note that in our results of Fig. 4 showing collective atomic migration along the domain boundaries, the net atomic motion through the junctions is of clockwise direction. The counterclockwise net atomic migration can also be obtained, simply by reversing grain orientations, as seen in two examples of Fig. S7a vs S7b. The corresponding grain shrinking behavior, i.e., $N$ vs $t$, is almost identical for both cases, as shown in Fig. 4c of the main text.

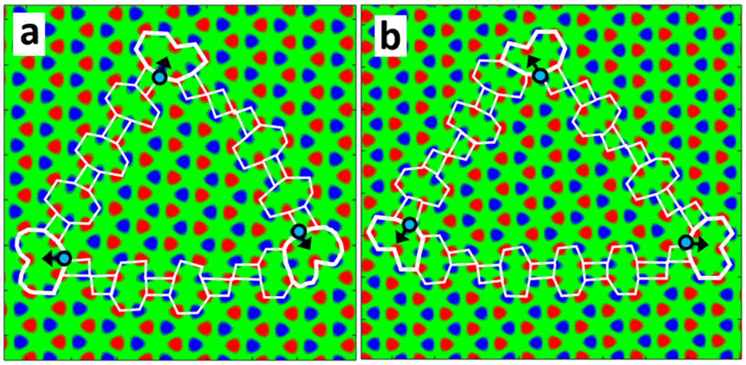


FIG. S7. Examples of two shrinking domains, with clockwise (a) and counterclockwise (b) net atomic motion through the junctions.

For the domain shrinking dynamics studied here, the growth exponent identified, i.e., $\alpha = 1/2$, is the same as that of purely curvature-driven growth. However, the underlying mechanism is expected to be different, based on the following 2 reasons: (i) The boundary lines of the inversion domain examined here are quite straight or weakly curved (mainly caused by the corners), as seen in Fig. 4, Fig. S7, and the supplemental movies. The motion of boundary lines is rigid and diffusionless, governed by the shape transformation of boundary defects via collective atomic displacement. (ii) For the cases of slower shrinking and stagnation of inversion domain with other types of domain boundary defects, we still obtain two regimes of linearly shrinking grain area (i.e., $\alpha = 1/2$; see Fig. S6) before the process becomes stagnant. This is very different from the previously studied systems of curved boundaries which yielded $\alpha < 1/2$ during grain growth and/or when approaching the grain stagnation regime. On the other hand, the previous results of $\alpha < 1/2$ and growth stagnation were mostly for polycrystalline systems with differently oriented grains, while here only a single grain orientation (i.e., for $60^\circ$ inversion domain) is examined. Thus the grain growth behavior observed here should be specific for the h-BN type binary systems with inversion symmetry breaking, particularly for the corresponding collective atomic-displacement dynamics of inversion domains. Our study for inversion domain growth will be useful for understanding its influence on the more complicated scenario of multi-grain dynamics in polycrystals of 2D binary materials.

[1] Z.-F. Huang, K. R. Elder, and N. Provatas, Phys. Rev. E **82**, 021605 (2010).
[2] K. R. Elder, M. Katakowski, M. Haataja, and M. Grant, Phys. Rev. Lett. **88**, 245701 (2002).
[3] Y. Liu, X. Zou, and B. I. Yakobson, ACS Nano **6**, 7053 (2012).
[4] O. V. Yazyev and S. G. Louie, Phys. Rev. B **81**, 195420 (2010).
[5] A. L. Gibb, N. Alem, J.-H. Chen, K. J. Erickson, J. Ciston, A. Gautam, M. Linck, and A. Zettl, J. Am. Chem. Soc. **135**, 6758 (2013).
[6] P. Hirvonen, M. M. Ervasti, Z. Fan, M. Jalalvand, M. Seymour, S. M. Vaez Allaei, N. Provatas, A. Harju, K. R. Elder, and T. Ala-Nissila, Phys. Rev. B **94**, 035414 (2016).
[7] T. Björkman, S. Kurasch, O. Lehtinen, J. Kotakoski, O. V. Yazyev, A. Srivastava, V. Skakalova, J. H. Smet, U. Kaiser, and A. V. Krasheninnikov, Sci. Rep. **3**, 3482 (2013).
[8] K. R. Elder and M. Grant, Phys. Rev. E **70**, 051605 (2004).
[9] X. Zou, Y. Liu, and B. I. Yakobson, Nano Lett. **13**, 253 (2013).
